# Supplementary material for: The First Fermi-LAT Catalog of Sources Above 10 GeV
Source: arXiv:1306.6772 ancillary file (2013-10-23)
Supplement: Supplementary file 2 [file Table7_Full_v2.pdf]

Table 1. Characteristics of the 1FHL Sources With AGN Associations

| 1FHL Name         | R.A.   | Decl.   | Assoc.                | Optical Class. | SED Class. | Redshift | Variability_BayesBlocks |
|-------------------|--------|---------|-----------------------|----------------|------------|----------|-------------------------|
| 1FHL J0007.7+4709 | 1.947  | 47.155  | MG4 J000800+4712      | BL Lac         | LSP        | 0.28&2.1 | 1                       |
| 1FHL J0008.7-2340 | 2.194  | -23.674 | RBS 0016              | BL Lac         | ...        | 0.147    | 1                       |
| 1FHL J0009.2+5032 | 2.316  | 50.541  | NVSS J000922+503028   | BL Lac         | ...        | ...      | 1                       |
| 1FHL J0018.6+2946 | 4.673  | 29.776  | RBS 0042              | BL Lac         | HSP        | ...      | 1                       |
| 1FHL J0022.2-1853 | 5.555  | -18.899 | 1RXS J002209.2-185333 | BL Lac         | HSP        | ...      | 1                       |
| 1FHL J0022.5+0607 | 5.643  | 6.124   | PKS 0019+058          | BL Lac         | LSP        | ...      | 1                       |
| 1FHL J0033.6-1921 | 8.407  | -19.361 | KUV 00311-1938        | BL Lac         | HSP        | 0.610    | 1                       |
| 1FHL J0035.2+1514 | 8.806  | 15.234  | RX J0035.2+1515       | BL Lac         | HSP        | ...      | 1                       |
| 1FHL J0035.9+5950 | 8.990  | 59.838  | 1ES 0033+595          | BL Lac         | HSP        | ...      | 1                       |
| 1FHL J0037.8+1238 | 9.473  | 12.645  | NVSS J003750+123818   | BL Lac         | HSP        | 0.089    | 1                       |
| 1FHL J0040.3+4049 | 10.096 | 40.827  | 1ES 0037+405          | BL Lac         | HSP        | ...      | 1                       |
| 1FHL J0043.7+3425 | 10.936 | 34.429  | GB6 J0043+3426        | FSRQ           | ...        | 0.966    | 1                       |
| 1FHL J0045.2+2126 | 11.310 | 21.448  | GB6 J0045+2127        | BL Lac         | HSP        | ...      | 1                       |
| 1FHL J0050.6-0930 | 12.672 | -9.510  | PKS 0048-09           | BL Lac         | ISP        | 0.635    | 1                       |
| 1FHL J0051.3-6240 | 12.846 | -62.672 | 1RXS J005117.7-624154 | AGU            | HSP        | ...      | 1                       |
| 1FHL J0054.8-2456 | 13.719 | -24.934 | 1RXS J005447.2-245532 | BL Lac         | HSP        | ...      | 1                       |
| 1FHL J0058.6-3236 | 14.663 | -32.610 | PKS 0055-328          | BL Lac         | LSP        | ...      | 1                       |
| 1FHL J0100.2+0747 | 15.073 | 7.785   | GB6 J0100+0745        | BL Lac         | ...        | ...      | 1                       |
| 1FHL J0103.4+5336 | 15.869 | 53.609  | 1RXS J010325.9+533721 | AGU            | HSP        | ...      | 1                       |
| 1FHL J0108.4+0134 | 17.105 | 1.577   | 4C +01.02             | FSRQ           | LSP        | 2.099    | 1                       |
| 1FHL J0110.3+6805 | 17.598 | 68.094  | 4C +67.04             | BL Lac         | ISP        | ...      | 1                       |
| 1FHL J0112.0+2244 | 18.010 | 22.748  | S2 0109+22            | BL Lac         | ISP        | 0.265    | 1                       |
| 1FHL J0112.9+3207 | 18.241 | 32.133  | 4C 31.03              | FSRQ           | LSP        | 0.603    | 1                       |
| 1FHL J0115.6+2520 | 18.906 | 25.333  | RX J0115.7+2519       | BL Lac         | HSP        | ...      | 1                       |
| 1FHL J0120.4-2701 | 20.115 | -27.024 | PKS 0118-272          | BL Lac         | LSP        | ...      | 1                       |
| 1FHL J0122.7+3425 | 20.682 | 34.418  | 1ES 0120+340          | BL Lac         | HSP        | 0.272    | 1                       |
| 1FHL J0131.3+6121 | 22.836 | 61.357  | 1RXS J013106.4+612035 | AGU            | HSP        | ...      | 1                       |
| 1FHL J0132.6-1651 | 23.165 | -16.859 | PKS 0130-17           | FSRQ           | LSP        | 1.020    | 1                       |
| 1FHL J0134.4+2643 | 23.602 | 26.733  | 1RXS J013427.2+263846 | AGU            | HSP        | ...      | 1                       |
| 1FHL J0136.5+3906 | 24.147 | 39.100  | B3 0133+388           | BL Lac         | HSP        | ...      | 1                       |
| 1FHL J0136.8+4754 | 24.208 | 47.901  | OC 457                | FSRQ           | LSP        | 0.859    | 1                       |
| 1FHL J0137.7+5812 | 24.436 | 58.216  | 1RXS J013748.0+581422 | AGU            | HSP        | ...      | 1                       |
| 1FHL J0141.5-0927 | 25.376 | -9.463  | PKS 0139-09           | BL Lac         | ISP        | 0.733    | 1                       |
| 1FHL J0143.4-5844 | 25.870 | -58.749 | SUMSS J014347-584550  | AGU            | HSP        | ...      | 1                       |
| 1FHL J0144.3+2703 | 26.084 | 27.064  | TXS 0141+268          | BL Lac         | LSP        | ...      | 1                       |

Table 1—Continued

| 1FHL Name         | R.A.   | Decl.   | Assoc.                          | Optical Class.  | SED Class. | Redshift      | Variability_BayesBlocks |
|-------------------|--------|---------|---------------------------------|-----------------|------------|---------------|-------------------------|
| 1FHL J0152.6+0148 | 28.163 | 1.800   | PMN J0152+0146                  | BL Lac          | HSP        | 0.080         | 1                       |
| 1FHL J0153.1+7515 | 28.287 | 75.258  | BZB J0153+7517                  | BL Lac          | HSP        | ...           | 1                       |
| 1FHL J0154.1+0823 | 28.527 | 8.390   | GB6 J0154+0823                  | BL Lac          | ISP        | 0.691         | 1                       |
| 1FHL J0156.5-2419 | 29.139 | -24.327 | TXS 0154-244                    | AGU             | ...        | ...           | 1                       |
| 1FHL J0159.4+1048 | 29.874 | 10.811  | RX J0159.5+1047                 | BL Lac          | HSP        | 0.195         | 1                       |
| 1FHL J0203.5+7232 | 30.891 | 72.533  | S5 0159+723                     | BL Lac          | LSP        | ...           | 1                       |
| 1FHL J0203.6+3042 | 30.904 | 30.702  | B2 0200+30                      | FSRQ            | ...        | 0.955         | 2                       |
| 1FHL J0208.7+3523 | 32.176 | 35.388  | BZB J0208+3523                  | BL Lac          | HSP        | 0.318         | 1                       |
| 1FHL J0209.6-5230 | 32.424 | -52.502 | 1RXS J020922.2-522920           | BL Lac          | HSP        | ...           | 1                       |
| 1FHL J0210.9-5100 | 32.737 | -51.002 | PKS 0208-512                    | AGU             | LSP        | 0.999         | 2                       |
| 1FHL J0211.3+1051 | 32.830 | 10.864  | MG1 J021114+1051                | BL Lac          | ISP        | ...           | 1                       |
| 1FHL J0213.1+2246 | 33.292 | 22.780  | MG3 J021252+2246                | BL Lac          | HSP        | 0.459         | 1                       |
| 1FHL J0217.4+0836 | 34.350 | 8.612   | BZB J0217+0837 & H 0214+0820    | BL Lac & FSRQ   | ISP & ...  | 0.085 & 2.000 | 1                       |
| 1FHL J0217.7+0142 | 34.444 | 1.701   | PKS 0215+015                    | FSRQ            | LSP        | 1.721         | 1                       |
| 1FHL J0221.1+3555 | 35.294 | 35.926  | S4 0218+35                      | FSRQ            | ...        | 0.944         | 1                       |
| 1FHL J0222.6+4302 | 35.669 | 43.035  | 3C 66A                          | BL Lac          | ISP        | ...           | 5                       |
| 1FHL J0237.5-3603 | 39.382 | -36.062 | RBS 0334                        | BL Lac          | HSP        | ...           | 1                       |
| 1FHL J0238.6-3117 | 39.657 | -31.284 | 1RXS J023832.6-311658           | BL Lac          | HSP        | 0.232         | 1                       |
| 1FHL J0238.7+1639 | 39.683 | 16.661  | AO 0235+164                     | BL Lac          | LSP        | 0.940         | 3                       |
| 1FHL J0241.3+6548 | 40.335 | 65.808  | NVSS J024121+654311             | AGU             | HSP        | ...           | 1                       |
| 1FHL J0244.2-5813 | 41.058 | -58.219 | BZB J0244-5819                  | BL Lac          | ...        | 0.264         | 1                       |
| 1FHL J0250.6+1712 | 42.657 | 17.206  | NVSS J025037+171209             | FSRQ            | HSP        | 1.100         | 1                       |
| 1FHL J0252.7-2218 | 43.177 | -22.311 | PKS 0250-225                    | FSRQ            | LSP        | 1.419         | 1                       |
| 1FHL J0303.4-2407 | 45.868 | -24.128 | PKS 0301-243                    | BL Lac          | HSP        | 0.260         | 3                       |
| 1FHL J0303.6+4715 | 45.922 | 47.266  | 4C +47.08                       | BL Lac          | LSP        | ...           | 1                       |
| 1FHL J0309.1+1027 | 47.290 | 10.459  | PKS 0306+102                    | FSRQ            | LSP        | 0.863         | 1                       |
| 1FHL J0310.5-5014 | 47.631 | -50.247 | SUMSS J031034-501633            | AGU             | HSP        | ...           | 1                       |
| 1FHL J0316.1+0904 | 49.035 | 9.068   | GB6 J0316+0904                  | BL Lac          | HSP        | ...           | 2                       |
| 1FHL J0316.3-2609 | 49.077 | -26.152 | RBS 0405                        | BL Lac          | HSP        | 0.443         | 1                       |
| 1FHL J0316.6+4119 | 49.169 | 41.322  | IC 310                          | Radio Gal       | ...        | 0.019         | 1                       |
| 1FHL J0318.8+2134 | 49.718 | 21.577  | J031846+213434                  | AGU             | ...        | ...           | 2                       |
| 1FHL J0319.8+1847 | 49.964 | 18.798  | RBS 0413                        | BL Lac          | HSP        | 0.190         | 1                       |
| 1FHL J0319.9+4130 | 49.977 | 41.508  | NGC 1275                        | Radio Gal       | ...        | 0.018         | 1                       |
| 1FHL J0322.1+2337 | 50.539 | 23.625  | MG3 J032201+2336                | BL Lac          | HSP        | ...           | 1                       |
| 1FHL J0323.5-0107 | 50.880 | -1.129  | BZB J0323-0111 & BZB J0323-0108 | BL Lac & BL Lac | HSP & HSP  | ... & 0.392   | 1                       |

Table 1—Continued

| 1FHL Name         | R.A.   | Decl.   | Assoc.                          | Optical Class. | SED Class. | Redshift      | Variability_BayesBlocks |
|-------------------|--------|---------|---------------------------------|----------------|------------|---------------|-------------------------|
| 1FHL J0325.7-1647 | 51.437 | -16.793 | RBS 0421                        | BL Lac         | HSP        | 0.291         | 1                       |
| 1FHL J0326.1+0224 | 51.545 | 2.413   | 1H 0323+022                     | BL Lac         | HSP        | 0.147         | 1                       |
| 1FHL J0333.6+2918 | 53.401 | 29.312  | TXS 0330+291                    | BL Lac         | ISP        | ...           | 1                       |
| 1FHL J0334.0+6539 | 53.505 | 65.666  | TXS 0329+654                    | BL Lac         | ISP        | ...           | 1                       |
| 1FHL J0334.1-4006 | 53.547 | -40.112 | PKS 0332-403                    | BL Lac         | ISP        | 1.357         | 1                       |
| 1FHL J0334.4-3726 | 53.604 | -37.443 | PMN J0334-3725                  | BL Lac         | LSP        | ...           | 1                       |
| 1FHL J0335.3-4501 | 53.846 | -45.029 | 1RXS J033514.5-445929           | AGU            | HSP        | ...           | 1                       |
| 1FHL J0338.1-2443 | 54.541 | -24.733 | BZB J0338-2443                  | BL Lac         | HSP        | 0.251         | 1                       |
| 1FHL J0423.3-0121 | 65.845 | -1.366  | PKS 0420-01                     | FSRQ           | LSP        | 0.916         | 1                       |
| 1FHL J0423.8+4151 | 65.951 | 41.851  | 4C +41.11                       | BL Lac         | ...        | ...           | 1                       |
| 1FHL J0428.7-3756 | 67.178 | -37.937 | PKS 0426-380                    | BL Lac         | LSP        | 1.111         | 3                       |
| 1FHL J0433.5+2905 | 68.389 | 29.086  | MG2 J043337+2905                | BL Lac         | LSP        | ...           | 1                       |
| 1FHL J0434.1-5725 | 68.537 | -57.428 | 1RXS J043431.8-572718           | AGU            | HSP        | ...           | 1                       |
| 1FHL J0442.9-0017 | 70.748 | -0.293  | BZQ J0442-0017 & BZB J0442-0018 | FSRQ & BL Lac  | LSP & ...  | 0.844 & 0.449 | 1                       |
| 1FHL J0448.5-1633 | 72.133 | -16.550 | RBS 0589                        | BL Lac         | HSP        | ...           | 1                       |
| 1FHL J0449.4-4350 | 72.361 | -43.840 | PKS 0447-439                    | BL Lac         | HSP        | 0.205         | 1                       |
| 1FHL J0457.1-2326 | 74.276 | -23.448 | PKS 0454-234                    | FSRQ           | ...        | 1.003         | 2                       |
| 1FHL J0505.4+0418 | 76.358 | 4.304   | MG1 J050533+0415                | BL Lac         | HSP        | ...           | 1                       |
| 1FHL J0506.9-5434 | 76.730 | -54.574 | 1ES 0505-546                    | AGU            | HSP        | ...           | 1                       |
| 1FHL J0508.1+6737 | 77.038 | 67.624  | 1ES 0502+675                    | BL Lac         | HSP        | 0.416&0.340   | 1                       |
| 1FHL J0509.5+0542 | 77.394 | 5.714   | TXS 0506+056                    | BL Lac         | ISP        | ...           | 2                       |
| 1FHL J0515.9+1528 | 78.985 | 15.469  | GB6 J0515+1527                  | BL Lac         | ...        | ...           | 1                       |
| 1FHL J0516.4+7351 | 79.124 | 73.852  | GB6 J0516+7350                  | BL Lac         | HSP        | 0.249         | 1                       |
| 1FHL J0516.6-6209 | 79.158 | -62.165 | PKS 0516-621                    | BL Lac         | ISP        | 1.300         | 1                       |
| 1FHL J0521.7+2113 | 80.449 | 21.220  | VER J0521+211                   | BL Lac         | ISP        | 0.108         | 1                       |
| 1FHL J0523.3-3620 | 80.847 | -36.339 | PKS 0521-36                     | AGU            | ...        | 0.055         | 1                       |
| 1FHL J0529.0+0937 | 82.272 | 9.618   | GB6 J0529+0934                  | AGU            | HSP        | ...           | 1                       |
| 1FHL J0532.1-4826 | 83.030 | -48.442 | PMN J0531-4827                  | AGU            | LSP        | ...           | 4                       |
| 1FHL J0536.4-3343 | 84.117 | -33.733 | 1RXS J053629.4-334302           | BL Lac         | HSP        | ...           | 1                       |
| 1FHL J0538.8-4405 | 84.713 | -44.088 | PKS 0537-441                    | BL Lac         | LSP        | 0.892         | 3                       |
| 1FHL J0540.5+5822 | 85.143 | 58.382  | GB6 J0540+5823                  | BL Lac         | HSP        | ...           | 1                       |
| 1FHL J0543.9-5532 | 85.981 | -55.538 | 1RXS J054357.3-553206           | BL Lac         | HSP        | ...           | 1                       |
| 1FHL J0550.6-3215 | 87.669 | -32.260 | PKS 0548-322                    | BL Lac         | HSP        | 0.069         | 1                       |
| 1FHL J0601.1-7037 | 90.296 | -70.623 | PKS 0601-70                     | FSRQ           | ...        | 2.409         | 1                       |
| 1FHL J0602.4-4013 | 90.620 | -40.221 | 1RXS J060251.9-4018351          | AGU            | ISP        | ...           | 1                       |

Table 1—Continued

| 1FHL Name         | R.A.    | Decl.   | Assoc.                     | Optical Class. | SED Class. | Redshift | Variability_BayesBlocks |
|-------------------|---------|---------|----------------------------|----------------|------------|----------|-------------------------|
| 1FHL J0604.2-4817 | 91.054  | -48.294 | 1ES 0602-482               | AGU            | HSP        | ...      | 1                       |
| 1FHL J0605.0+0001 | 91.258  | 0.032   | GB6 J0604+0000             | AGU            | ...        | ...      | 1                       |
| 1FHL J0606.6+4742 | 91.655  | 47.710  | CGRaBS_J0607+4739          | BL Lac         | ...        | ...      | 1                       |
| 1FHL J0609.4-0248 | 92.375  | -2.812  | NVSS J060915-024754        | BL Lac         | HSP        | ...      | 1                       |
| 1FHL J0612.8+4121 | 93.202  | 41.365  | B3 0609+413                | BL Lac         | ...        | ...      | 1                       |
| 1FHL J0617.0+5700 | 94.270  | 57.012  | 87GB 061258.1+570222       | BL Lac         | ISP        | ...      | 1                       |
| 1FHL J0617.6-1716 | 94.413  | -17.281 | CRATES J061733.67-171522.8 | BL Lac         | LSP        | 0.098    | 1                       |
| 1FHL J0622.4-2604 | 95.604  | -26.072 | CRATES J0622-2606          | AGU            | ...        | 0.414    | 1                       |
| 1FHL J0622.9+3328 | 95.730  | 33.469  | B2 0619+33                 | AGU            | ...        | ...      | 3                       |
| 1FHL J0625.3+4440 | 96.338  | 44.668  | GB6 J0625+4440             | BL Lac         | ...        | ...      | 1                       |
| 1FHL J0626.8-3528 | 96.704  | -35.479 | PKS 0625-35                | Radio Gal      | ...        | 0.055    | 1                       |
| 1FHL J0630.9-2406 | 97.748  | -24.113 | TXS 0628-240               | BL Lac         | HSP        | ...      | 1                       |
| 1FHL J0644.2-6713 | 101.053 | -67.220 | PKS 0644-671               | AGU            | ...        | ...      | 2                       |
| 1FHL J0647.1-5131 | 101.798 | -51.525 | 1RXS J064710.1-513546      | AGU            | HSP        | ...      | 1                       |
| 1FHL J0648.9+1516 | 102.225 | 15.281  | VER J0648+152              | BL Lac         | HSP        | 0.179    | 1                       |
| 1FHL J0649.5-3138 | 102.395 | -31.647 | 1RXS J064933.8-313914      | AGU            | HSP        | ...      | 1                       |
| 1FHL J0650.8+2504 | 102.712 | 25.081  | 1ES 0647+250               | BL Lac         | HSP        | ...      | 1                       |
| 1FHL J0654.2+4514 | 103.568 | 45.244  | B3 0650+453                | FSRQ           | LSP        | 0.928    | 1                       |
| 1FHL J0654.5+5042 | 103.647 | 50.706  | GB6 J0654+5042             | FSRQ           | LSP        | 1.253    | 1                       |
| 1FHL J0700.6-6612 | 105.168 | -66.202 | PKS 0700-661               | BL Lac         | ISP        | ...      | 1                       |
| 1FHL J0706.5+3744 | 106.649 | 37.749  | GB6 J0706+3744             | BL Lac         | HSP        | ...      | 1                       |
| 1FHL J0710.5+5908 | 107.629 | 59.139  | 1H 0658+595                | BL Lac         | HSP        | 0.125    | 1                       |
| 1FHL J0712.8+5034 | 108.210 | 50.571  | GB6 J0712+5033             | BL Lac         | LSP        | 0.502    | 1                       |
| 1FHL J0718.7-4321 | 109.691 | -43.363 | PMN J0718-4319             | BL Lac         | ISP        | ...      | 1                       |
| 1FHL J0719.2+3308 | 109.819 | 33.141  | B2 0716+33                 | FSRQ           | LSP        | 0.779    | 1                       |
| 1FHL J0721.8+7120 | 110.461 | 71.339  | S5 0716+71                 | BL Lac         | ISP        | ...      | 2                       |
| 1FHL J0725.2+1423 | 111.316 | 14.393  | 4C +14.23                  | FSRQ           | LSP        | 1.038    | 3                       |
| 1FHL J0730.2+3307 | 112.568 | 33.127  | 1RXS J073026.0+330727      | BL Lac         | HSP        | 0.112    | 1                       |
| 1FHL J0730.3-1140 | 112.577 | -11.673 | PKS 0727-11                | FSRQ           | ...        | 1.591    | 1                       |
| 1FHL J0735.0-7708 | 113.774 | -77.137 | PKS 0736-770               | AGU            | LSP        | ...      | 1                       |
| 1FHL J0738.0+1742 | 114.507 | 17.701  | PKS 0735+17                | BL Lac         | LSP        | 0.424    | 1                       |
| 1FHL J0743.0+5446 | 115.773 | 54.777  | GB6 J0742+5444             | FSRQ           | LSP        | 0.723    | 1                       |
| 1FHL J0745.2+7439 | 116.304 | 74.650  | MS 0737.9+7441             | BL Lac         | HSP        | 0.315    | 1                       |
| 1FHL J0745.2+8511 | 116.315 | 85.192  | NVSS J074715+851208        | AGU            | HSP        | ...      | 1                       |
| 1FHL J0746.3-4757 | 116.587 | -47.951 | CRATES J0746-4754          | AGU            | ISP        | ...      | 1                       |

Table 1—Continued

| 1FHL Name         | R.A.    | Decl.   | Assoc.                | Optical Class. | SED Class. | Redshift             | Variability_BayesBlocks |
|-------------------|---------|---------|-----------------------|----------------|------------|----------------------|-------------------------|
| 1FHL J0747.1-3315 | 116.779 | -33.261 | J074719-331046        | AGU            | ...        | ...                  | 1                       |
| 1FHL J0753.0+5351 | 118.269 | 53.852  | 4C +54.15             | BL Lac         | LSP        | 0.730                | 1                       |
| 1FHL J0754.3-1149 | 118.599 | -11.824 | TXS 0752-116          | BL Lac         | ...        | ...                  | 1                       |
| 1FHL J0757.2+0955 | 119.322 | 9.918   | PKS 0754+100          | BL Lac         | ISP        | 0.266                | 1                       |
| 1FHL J0805.4+7534 | 121.369 | 75.575  | RX J0805.4+7534       | BL Lac         | HSP        | 0.121                | 1                       |
| 1FHL J0807.1-0543 | 121.782 | -5.723  | PKS 0804-05           | BL Lac         | ...        | ...                  | 1                       |
| 1FHL J0808.2-0749 | 122.070 | -7.823  | PKS 0805-07           | FSRQ           | LSP        | 1.837                | 3                       |
| 1FHL J0809.8+5217 | 122.461 | 52.294  | 1ES 0806+524          | BL Lac         | HSP        | 0.137                | 2                       |
| 1FHL J0811.1-7525 | 122.786 | -75.433 | PMN J0810-7530        | BL Lac         | ISP        | ...                  | 1                       |
| 1FHL J0811.4+0149 | 122.861 | 1.825   | OJ 014                | BL Lac         | LSP        | 1.148                | 1                       |
| 1FHL J0816.3-1310 | 124.091 | -13.177 | PMN J0816-1311        | BL Lac         | HSP        | ...                  | 1                       |
| 1FHL J0817.9+4224 | 124.498 | 42.416  | S4 0814+42            | BL Lac         | LSP        | ...                  | 1                       |
| 1FHL J0818.0-0935 | 124.507 | -9.585  | TXS 0815-094          | BL Lac         | ...        | ...                  | 1                       |
| 1FHL J0825.9+0308 | 126.478 | 3.144   | PKS 0823+033          | BL Lac         | ISP        | 0.506                | 1                       |
| 1FHL J0826.0-2230 | 126.502 | -22.517 | PKS 0823-223          | BL Lac         | ISP        | 0.910                | 1                       |
| 1FHL J0832.0+0429 | 128.000 | 4.484   | PKS 0829+046          | BL Lac         | LSP        | 0.174                | 1                       |
| 1FHL J0845.8-5553 | 131.455 | -55.894 | AT20G J084549-555528  | AGU            | ...        | ...                  | 1                       |
| 1FHL J0846.8-2338 | 131.706 | -23.640 | PMN J0847-2337        | BL Lac         | ...        | 0.059                | 1                       |
| 1FHL J0847.0+1132 | 131.773 | 11.544  | RX J0847.1+1133       | BL Lac         | HSP        | 0.198                | 1                       |
| 1FHL J0850.0+4849 | 132.512 | 48.819  | GB6 J0850+4855        | BL Lac         | ISP        | ...                  | 1                       |
| 1FHL J0850.2-1211 | 132.554 | -12.189 | BZQ J0850-1213        | FSRQ           | LSP        | 0.566                | 1                       |
| 1FHL J0852.9-3656 | 133.249 | -36.945 | NVSS J085310-365820   | AGU            | ...        | ...                  | 1                       |
| 1FHL J0854.8+2004 | 133.712 | 20.079  | OJ 287                | BL Lac         | ISP        | 0.306                | 1                       |
| 1FHL J0856.7-1106 | 134.199 | -11.115 | CRATES J0856-1105     | BL Lac         | LSP        | ...                  | 1                       |
| 1FHL J0905.6+1359 | 136.415 | 13.986  | MG1 J090534+1358      | BL Lac         | ...        | ...                  | 1                       |
| 1FHL J0909.3+2312 | 137.339 | 23.205  | RX J0908.9+2311       | BL Lac         | HSP        | 0.223&LowLimit_0.431 | 1                       |
| 1FHL J0910.6+3333 | 137.668 | 33.555  | Ton 1015              | BL Lac         | HSP        | ...                  | 1                       |
| 1FHL J0912.5+2758 | 138.132 | 27.974  | 1RXS J091211.9+275955 | BL Lac         | HSP        | ...                  | 1                       |
| 1FHL J0913.1-2104 | 138.289 | -21.078 | MRC 0910-208          | BL Lac         | HSP        | 0.198                | 1                       |
| 1FHL J0915.8+2932 | 138.975 | 29.549  | B2 0912+29            | BL Lac         | HSP        | ...                  | 1                       |
| 1FHL J0920.9+4443 | 140.230 | 44.731  | S4 0917+44            | FSRQ           | LSP        | 2.189                | 1                       |
| 1FHL J0929.5+5014 | 142.394 | 50.240  | GB6 J0929+5013        | BL Lac         | ISP        | ...                  | 1                       |
| 1FHL J0930.4+8611 | 142.617 | 86.197  | S5 0916+864           | BL Lac         | LSP        | ...                  | 1                       |
| 1FHL J0946.2+0106 | 146.574 | 1.105   | RXS J094620.5+010459  | BL Lac         | HSP        | 0.557                | 1                       |
| 1FHL J0952.9-0839 | 148.238 | -8.655  | PMN J0953-0840        | BL Lac         | HSP        | ...                  | 1                       |

Table 1—Continued

| 1FHL Name         | R.A.    | Decl.   | Assoc.                | Optical Class. | SED Class. | Redshift | Variability_BayesBlocks |
|-------------------|---------|---------|-----------------------|----------------|------------|----------|-------------------------|
| 1FHL J0957.6+5522 | 149.421 | 55.377  | 4C +55.17             | FSRQ           | LSP        | 0.899    | 1                       |
| 1FHL J0959.5+6535 | 149.884 | 65.585  | S4 0954+65            | BL Lac         | ISP        | 0.367    | 1                       |
| 1FHL J1009.6-3118 | 152.414 | -31.302 | 1RXS J101015.9-311909 | BL Lac         | HSP        | 0.143    | 1                       |
| 1FHL J1015.0+4925 | 153.773 | 49.427  | 1H 1013+498           | BL Lac         | HSP        | 0.212    | 1                       |
| 1FHL J1016.0+0512 | 154.010 | 5.205   | TXS 1013+054          | FSRQ           | ...        | 1.714    | 2                       |
| 1FHL J1023.6+2959 | 155.909 | 29.995  | RX J1023.6+3001       | BL Lac         | HSP        | 0.433    | 1                       |
| 1FHL J1023.9-4337 | 155.979 | -43.618 | RX J1023.9-4336       | BL Lac         | HSP        | ...      | 1                       |
| 1FHL J1029.0-8543 | 157.253 | -85.730 | PKS 1029-85           | BL Lac         | LSP        | ...      | 1                       |
| 1FHL J1031.0+5052 | 157.759 | 50.879  | 1ES 1028+511          | BL Lac         | HSP        | ...      | 1                       |
| 1FHL J1033.7+6051 | 158.435 | 60.858  | S4 1030+61            | FSRQ           | LSP        | 1.401    | 2                       |
| 1FHL J1037.4+5712 | 159.374 | 57.201  | GB6 J1037+5711        | BL Lac         | ISP        | ...      | 1                       |
| 1FHL J1043.2+2407 | 160.822 | 24.119  | B2 1040+24A           | BL Lac         | ISP        | 0.559    | 1                       |
| 1FHL J1048.3+7241 | 162.082 | 72.686  | GB6 J1047+7238        | BL Lac         | ...        | ...      | 1                       |
| 1FHL J1053.6+4931 | 163.403 | 49.521  | GB6 J1053+4930        | BL Lac         | HSP        | 0.140    | 1                       |
| 1FHL J1054.6+2214 | 163.671 | 22.234  | 87GB 105148.6+222705  | BL Lac         | ISP        | ...      | 1                       |
| 1FHL J1058.5+0133 | 164.628 | 1.563   | 4C +01.28             | BL Lac         | LSP        | 0.888    | 1                       |
| 1FHL J1058.6+5627 | 164.666 | 56.459  | TXS 1055+567          | BL Lac         | HSP        | 0.143    | 1                       |
| 1FHL J1058.8-1134 | 164.703 | -11.570 | PKS B1056-113         | BL Lac         | LSP        | ...      | 1                       |
| 1FHL J1100.6+4018 | 165.165 | 40.315  | RX J1100.3+4019       | BL Lac         | HSP        | 0.225    | 1                       |
| 1FHL J1103.3-2329 | 165.846 | -23.492 | 1ES 1101-232          | BL Lac         | HSP        | 0.186    | 1                       |
| 1FHL J1104.2-5356 | 166.064 | -53.942 | PKS 1101-536          | BL Lac         | LSP        | ...      | 1                       |
| 1FHL J1104.4+3812 | 166.121 | 38.207  | Mkn 421               | BL Lac         | HSP        | 0.031    | 1                       |
| 1FHL J1107.5+0223 | 166.878 | 2.386   | BZB J1107+0222        | BL Lac         | ...        | ...      | 1                       |
| 1FHL J1117.2+2013 | 169.305 | 20.227  | RBS 0958              | BL Lac         | HSP        | 0.138    | 1                       |
| 1FHL J1117.7+5355 | 169.445 | 53.933  | BZB J1117+5355        | BL Lac         | HSP        | ...      | 1                       |
| 1FHL J1120.9+4211 | 170.245 | 42.190  | RBS 0970              | BL Lac         | HSP        | ...      | 1                       |
| 1FHL J1125.9-3557 | 171.496 | -35.956 | PMN J1125-3556        | BL Lac         | ISP        | 0.284    | 1                       |
| 1FHL J1127.1-1855 | 171.793 | -18.933 | PKS 1124-186          | FSRQ           | LSP        | 1.048    | 2                       |
| 1FHL J1130.4+5814 | 172.603 | 58.234  | BZB J1131+5809        | BL Lac         | ISP        | 0.360    | 1                       |
| 1FHL J1132.6+0036 | 173.165 | 0.603   | PKS B1130+008         | BL Lac         | ISP        | 0.678    | 1                       |
| 1FHL J1135.7+6736 | 173.939 | 67.612  | RX J1136.5+6737       | BL Lac         | HSP        | 0.134    | 1                       |
| 1FHL J1136.4+7009 | 174.100 | 70.159  | Mkn 180               | BL Lac         | HSP        | 0.046    | 1                       |
| 1FHL J1137.0+2553 | 174.267 | 25.893  | RX J1136.8+2551       | BL Lac         | HSP        | 0.156    | 1                       |
| 1FHL J1146.9+3958 | 176.747 | 39.978  | S4 1144+40            | FSRQ           | ...        | 1.088    | 1                       |
| 1FHL J1150.5+4155 | 177.649 | 41.917  | RBS 1040              | BL Lac         | HSP        | ...      | 1                       |

Table 1—Continued

| 1FHL Name         | R.A.    | Decl.   | Assoc.                | Optical Class. | SED Class. | Redshift    | Variability_BayesBlocks |
|-------------------|---------|---------|-----------------------|----------------|------------|-------------|-------------------------|
| 1FHL J1150.8+2419 | 177.711 | 24.320  | B2 1147+24            | BL Lac         | LSP        | 0.200       | 1                       |
| 1FHL J1151.5+5857 | 177.880 | 58.958  | TXS 1148+592          | BL Lac         | ISP        | ...         | 1                       |
| 1FHL J1154.0-0010 | 178.525 | -0.169  | 1RXS J115404.9-001008 | BL Lac         | HSP        | 0.254       | 1                       |
| 1FHL J1159.6+2913 | 179.919 | 29.227  | Ton 599               | FSRQ           | LSP        | 0.725       | 1                       |
| 1FHL J1203.2+6028 | 180.807 | 60.471  | SBS 1200+608          | BL Lac         | ISP        | 0.065       | 1                       |
| 1FHL J1204.4-0708 | 181.103 | -7.142  | 1RXS J120417.0-070959 | BL Lac         | ISP        | 0.184       | 1                       |
| 1FHL J1217.8+3006 | 184.460 | 30.105  | 1ES 1215+303          | BL Lac         | HSP        | 0.130       | 1                       |
| 1FHL J1221.3+3011 | 185.337 | 30.194  | PG 1218+304           | BL Lac         | HSP        | 0.184       | 1                       |
| 1FHL J1221.6+2814 | 185.402 | 28.247  | W Comae               | BL Lac         | ISP        | 0.103       | 1                       |
| 1FHL J1224.5+2437 | 186.146 | 24.628  | MS 1221.8+2452        | BL Lac         | HSP        | 0.218       | 1                       |
| 1FHL J1224.8+2122 | 186.220 | 21.377  | 4C +21.35             | FSRQ           | LSP        | 0.434       | 10                      |
| 1FHL J1228.5+4857 | 187.146 | 48.960  | TXS 1226+492          | FSRQ           | LSP        | 1.722       | 1                       |
| 1FHL J1230.3+2522 | 187.586 | 25.377  | ON 246                | BL Lac         | ISP        | 0.135       | 1                       |
| 1FHL J1230.8+1224 | 187.701 | 12.406  | M 87                  | Radio Gal      | ...        | 0.004       | 1                       |
| 1FHL J1231.8+2849 | 187.970 | 28.825  | B2 1229+29            | BL Lac         | HSP        | 0.236       | 1                       |
| 1FHL J1234.1-5735 | 188.531 | -57.592 | PMN J1234-5736        | AGU            | ...        | ...         | 1                       |
| 1FHL J1239.6+0443 | 189.901 | 4.732   | MG1 J123931+0443      | FSRQ           | LSP        | 1.761       | 1                       |
| 1FHL J1243.2+3628 | 190.807 | 36.468  | Ton 116               | BL Lac         | HSP        | 1.065       | 1                       |
| 1FHL J1244.9+5708 | 191.244 | 57.140  | 1RXS J124510.5+571020 | BL Lac         | ISP        | ...         | 1                       |
| 1FHL J1246.6-2548 | 191.659 | -25.809 | PKS 1244-255          | FSRQ           | LSP        | 0.633       | 1                       |
| 1FHL J1248.1+5821 | 192.041 | 58.361  | PG 1246+586           | BL Lac         | ISP        | 0.847       | 1                       |
| 1FHL J1249.7+3706 | 192.427 | 37.102  | RX J1249.8+3708       | BL Lac         | HSP        | ...         | 1                       |
| 1FHL J1253.1+5301 | 193.294 | 53.020  | S4 1250+53            | BL Lac         | ISP        | ...         | 1                       |
| 1FHL J1253.6+0329 | 193.423 | 3.491   | CRATES J1253+0326     | BL Lac         | ...        | ...         | 1                       |
| 1FHL J1256.1-0547 | 194.049 | -5.798  | 3C 279                | FSRQ           | LSP        | 0.536       | 2                       |
| 1FHL J1256.4-1146 | 194.112 | -11.770 | PMN J1256-1146        | AGU            | ...        | 0.058       | 1                       |
| 1FHL J1302.9+2433 | 195.748 | 24.563  | MG2 J130304+2434      | BL Lac         | ...        | 0.993       | 1                       |
| 1FHL J1304.1-2413 | 196.048 | -24.230 | 1RXS J130343.6-241506 | AGU            | HSP        | 0.127       | 1                       |
| 1FHL J1304.3-4354 | 196.080 | -43.915 | 1RXS J130421.2-435308 | BL Lac         | HSP        | ...         | 1                       |
| 1FHL J1307.7-4259 | 196.929 | -42.999 | 1RXS J130737.8-425940 | AGU            | HSP        | ...         | 1                       |
| 1FHL J1309.3+4304 | 197.345 | 43.069  | B3 1307+433           | BL Lac         | HSP        | 0.691       | 1                       |
| 1FHL J1310.6+3222 | 197.674 | 32.381  | OP 313                | FSRQ           | LSP        | 0.997       | 1                       |
| 1FHL J1310.9+0036 | 197.740 | 0.607   | RX J1311.1+0035       | BL Lac         | HSP        | ...         | 1                       |
| 1FHL J1312.2-2158 | 198.061 | -21.970 | PKS 1309-216          | BL Lac         | ...        | 1.491&1.600 | 1                       |
| 1FHL J1312.8+4827 | 198.201 | 48.459  | GB 1310+487           | FSRQ           | LSP        | 0.501       | 3                       |

Table 1—Continued

| 1FHL Name         | R.A.    | Decl.   | Assoc.                | Optical Class. | SED Class. | Redshift | Variability_BayesBlocks |
|-------------------|---------|---------|-----------------------|----------------|------------|----------|-------------------------|
| 1FHL J1314.9-4241 | 198.749 | -42.696 | MS 13121-4221         | BL Lac         | HSP        | 0.108    | 1                       |
| 1FHL J1315.0+2346 | 198.772 | 23.773  | TXS 1312+240          | BL Lac         | ISP        | ...      | 1                       |
| 1FHL J1315.9-3333 | 198.993 | -33.559 | PKS 1313-333          | FSRQ           | LSP        | 1.210    | 1                       |
| 1FHL J1322.9+2942 | 200.731 | 29.702  | 4C +29.48             | AGU            | ...        | ...      | 1                       |
| 1FHL J1326.1-4303 | 201.528 | -43.054 | Cen A Core            | Radio Gal      | ...        | 0.002    | 1                       |
| 1FHL J1327.1-5258 | 201.788 | -52.974 | PMN J1326-5256        | BL Lac         | LSP        | ...      | 1                       |
| 1FHL J1328.7-5604 | 202.195 | -56.079 | PMN J1329-5608        | AGU            | LSP        | ...      | 1                       |
| 1FHL J1330.4-7005 | 202.615 | -70.084 | PKS 1326-697          | AGU            | ...        | ...      | 1                       |
| 1FHL J1332.0-0508 | 203.015 | -5.136  | PKS 1329-049          | FSRQ           | LSP        | 2.150    | 1                       |
| 1FHL J1344.0-1722 | 206.001 | -17.381 | PMN J1344-1723        | FSRQ           | ...        | 2.506    | 1                       |
| 1FHL J1351.4+1115 | 207.867 | 11.256  | RX J1351.3+1115       | BL Lac         | HSP        | ...      | 1                       |
| 1FHL J1359.9-3746 | 209.987 | -37.777 | PMN J1359-3746        | BL Lac         | ...        | 0.334    | 1                       |
| 1FHL J1406.3-2509 | 211.585 | -25.157 | NVSS J140609-250808   | AGU            | ...        | ...      | 1                       |
| 1FHL J1418.4-0234 | 214.603 | -2.574  | BZB J1418-0233        | BL Lac         | ...        | ...      | 1                       |
| 1FHL J1418.6+2539 | 214.659 | 25.658  | BZB J1417+2543        | BL Lac         | HSP        | 0.237    | 1                       |
| 1FHL J1419.0+7730 | 214.755 | 77.505  | 1RXS J141901.8+773229 | AGU            | HSP        | ...      | 1                       |
| 1FHL J1425.1+3613 | 216.288 | 36.219  | BZB J1424+3615        | BL Lac         | ISP        | ...      | 1                       |
| 1FHL J1427.0+2347 | 216.766 | 23.790  | PKS 1424+240          | BL Lac         | HSP        | ...      | 1                       |
| 1FHL J1428.0-4206 | 217.012 | -42.104 | PKS B1424-418         | FSRQ           | LSP        | 1.522    | 2                       |
| 1FHL J1428.6+4239 | 217.158 | 42.659  | H 1426+428            | BL Lac         | HSP        | 0.129    | 1                       |
| 1FHL J1436.9+5642 | 219.243 | 56.702  | BZB J1436+5639        | BL Lac         | HSP        | ...      | 1                       |
| 1FHL J1439.3+3933 | 219.835 | 39.555  | PG 1437+398           | BL Lac         | HSP        | 0.349    | 1                       |
| 1FHL J1441.0+0609 | 220.252 | 6.162   | PMN J1440+0610        | BL Lac         | ISP        | ...      | 1                       |
| 1FHL J1442.9+1158 | 220.737 | 11.982  | 1ES 1440+122          | BL Lac         | HSP        | 0.163    | 1                       |
| 1FHL J1444.0-3908 | 221.011 | -39.145 | PKS 1440-389          | BL Lac         | HSP        | 0.065    | 1                       |
| 1FHL J1448.2+3607 | 222.052 | 36.123  | RBS 1432              | BL Lac         | HSP        | ...      | 1                       |
| 1FHL J1454.4+5120 | 223.619 | 51.336  | TXS 1452+516          | BL Lac         | ISP        | ...      | 1                       |
| 1FHL J1457.3-3544 | 224.341 | -35.741 | PKS 1454-354          | FSRQ           | LSP        | 1.424    | 2                       |
| 1FHL J1501.0+2238 | 225.275 | 22.639  | MS 1458.8+2249        | BL Lac         | HSP        | 0.235    | 1                       |
| 1FHL J1503.9-1540 | 225.976 | -15.681 | RBS 1457              | BL Lac         | ...        | ...      | 1                       |
| 1FHL J1504.3+1029 | 226.095 | 10.488  | PKS 1502+106          | FSRQ           | LSP        | 1.839    | 2                       |
| 1FHL J1512.2+0204 | 228.064 | 2.074   | PKS 1509+022          | FSRQ           | LSP        | 0.219    | 1                       |
| 1FHL J1512.8-0906 | 228.201 | -9.111  | PKS 1510-08           | FSRQ           | LSP        | 0.360    | 3                       |
| 1FHL J1517.8-2421 | 229.453 | -24.357 | AP Librae             | BL Lac         | LSP        | 0.048    | 1                       |
| 1FHL J1517.9+6526 | 229.480 | 65.448  | 1H 1515+660           | BL Lac         | HSP        | 0.702    | 1                       |



Table 1—Continued

| 1FHL Name         | R.A.    | Decl.   | Assoc.                | Optical Class. | SED Class. | Redshift | Variability_BayesBlocks |
|-------------------|---------|---------|-----------------------|----------------|------------|----------|-------------------------|
| 1FHL J1518.4-2733 | 229.610 | -27.550 | TXS 1515-273          | AGU            | ...        | ...      | 1                       |
| 1FHL J1520.8-0348 | 230.210 | -3.806  | NVSS J152048-034850   | BL Lac         | HSP        | ...      | 1                       |
| 1FHL J1522.2+3145 | 230.554 | 31.754  | B2 1520+31            | FSRQ           | LSP        | 1.484    | 1                       |
| 1FHL J1532.6-1317 | 233.166 | -13.299 | CGRaBS J1532-1319     | AGU            | ...        | ...      | 2                       |
| 1FHL J1537.5+8159 | 234.395 | 81.989  | 1ES 1544+820          | BL Lac         | HSP        | ...      | 1                       |
| 1FHL J1542.9+6128 | 235.726 | 61.478  | GB6 J1542+6129        | BL Lac         | ISP        | ...      | 1                       |
| 1FHL J1548.8-2251 | 237.224 | -22.854 | PMN J1548-2251        | BL Lac         | HSP        | 0.192    | 1                       |
| 1FHL J1553.4-3117 | 238.362 | -31.295 | 1RXS J155333.4-311841 | BL Lac         | HSP        | ...      | 1                       |
| 1FHL J1555.7+1111 | 238.942 | 11.190  | PG 1553+113           | BL Lac         | HSP        | ...      | 2                       |
| 1FHL J1558.5-6428 | 239.645 | -64.481 | PMN J1558-6432        | AGU            | ISP        | 0.080    | 1                       |
| 1FHL J1603.7-4903 | 240.950 | -49.063 | PMN J1603-4904        | BL Lac         | LSP        | ...      | 2                       |
| 1FHL J1610.9-6650 | 242.726 | -66.849 | PMN J1610-6649        | BL Lac         | HSP        | ...      | 1                       |
| 1FHL J1625.7-2531 | 246.433 | -25.517 | PKS 1622-253          | FSRQ           | ...        | 0.786    | 1                       |
| 1FHL J1631.0+5224 | 247.771 | 52.401  | TXS 1629+524          | BL Lac         | ISP        | ...      | 1                       |
| 1FHL J1635.0+3808 | 248.767 | 38.143  | 4C +38.41             | FSRQ           | LSP        | 1.813    | 2                       |
| 1FHL J1637.9-3450 | 249.482 | -34.838 | NVSS J163750-344915   | AGU            | HSP        | ...      | 1                       |
| 1FHL J1640.7+3943 | 250.197 | 39.730  | NRAO 512              | FSRQ           | LSP        | 1.660    | 1                       |
| 1FHL J1650.1-5045 | 252.530 | -50.757 | PMN J1650-5044        | AGU            | ...        | ...      | 1                       |
| 1FHL J1653.9+3945 | 253.489 | 39.754  | Mkn 501               | BL Lac         | HSP        | 0.034    | 1                       |
| 1FHL J1709.5+4320 | 257.393 | 43.349  | B3 1708+433           | FSRQ           | LSP        | 1.027    | 1                       |
| 1FHL J1719.1+1745 | 259.798 | 17.750  | PKS 1717+177          | BL Lac         | LSP        | 0.137    | 2                       |
| 1FHL J1722.6+1011 | 260.654 | 10.198  | TXS 1720+102          | FSRQ           | LSP        | 0.732    | 1                       |
| 1FHL J1725.1+1151 | 261.293 | 11.866  | 1H 1720+117           | BL Lac         | HSP        | ...      | 1                       |
| 1FHL J1728.3+5014 | 262.089 | 50.236  | 1es 1727+502          | BL Lac         | HSP        | 0.055    | 1                       |
| 1FHL J1730.7+0017 | 262.700 | 0.297   | PKS 1728+004          | FSRQ           | ...        | 1.335    | 1                       |
| 1FHL J1735.3-1118 | 263.840 | -11.311 | CRATES J1735-1117     | AGU            | ...        | ...      | 1                       |
| 1FHL J1735.9+2033 | 263.999 | 20.552  | NVSS J173605+203301   | BL Lac         | HSP        | ...      | 1                       |
| 1FHL J1739.3+4953 | 264.846 | 49.884  | S4 1738+49            | FSRQ           | LSP        | 1.545    | 1                       |
| 1FHL J1740.2+5211 | 265.071 | 52.184  | 4C +51.37             | FSRQ           | LSP        | 1.379    | 1                       |
| 1FHL J1744.2+1938 | 266.058 | 19.641  | 1es 1741+196          | BL Lac         | HSP        | 0.083    | 1                       |
| 1FHL J1748.5+7006 | 267.127 | 70.101  | S4 1749+70            | BL Lac         | ISP        | 0.770    | 2                       |
| 1FHL J1751.5+0938 | 267.876 | 9.640   | OT 081                | BL Lac         | LSP        | 0.322    | 1                       |
| 1FHL J1754.2+3213 | 268.560 | 32.224  | RX J1754.1+3212       | BL Lac         | HSP        | ...      | 2                       |
| 1FHL J1756.5+5523 | 269.138 | 55.393  | 1RXS J175615.5+552217 | BL Lac         | HSP        | ...      | 1                       |
| 1FHL J1800.5+7829 | 270.147 | 78.483  | S5 1803+784           | BL Lac         | LSP        | 0.680    | 1                       |

Table 1—Continued

| 1FHL Name         | R.A.    | Decl.   | Assoc.                | Optical Class. | SED Class. | Redshift             | Variability_BayesBlocks |
|-------------------|---------|---------|-----------------------|----------------|------------|----------------------|-------------------------|
| 1FHL J1802.7-3940 | 270.680 | -39.674 | PMN J1802-3940        | FSRQ           | LSP        | 1.319                | 1                       |
| 1FHL J1806.3+6948 | 271.586 | 69.802  | 3C 371                | BL Lac         | ISP        | 0.051                | 1                       |
| 1FHL J1809.3+2040 | 272.336 | 20.680  | RX J1809.3+2041       | BL Lac         | HSP        | ...                  | 1                       |
| 1FHL J1809.6+2910 | 272.410 | 29.167  | MG2 J180948+2910      | BL Lac         | ...        | ...                  | 1                       |
| 1FHL J1813.4+3145 | 273.371 | 31.752  | B2 1811+31            | BL Lac         | ISP        | 0.117                | 1                       |
| 1FHL J1823.7-3455 | 275.929 | -34.919 | NVSS J182338-345412   | AGU            | ...        | ...                  | 1                       |
| 1FHL J1828.9-2417 | 277.246 | -24.284 | 1RXS J182853.8-241746 | AGU            | HSP        | ...                  | 1                       |
| 1FHL J1833.7-2105 | 278.428 | -21.087 | PKS 1830-211          | FSRQ           | ...        | 2.507                | 1                       |
| 1FHL J1838.8+4800 | 279.713 | 48.012  | GB6 J1838+4802        | BL Lac         | HSP        | ...                  | 1                       |
| 1FHL J1841.8+3219 | 280.465 | 32.330  | RX J1841.7+3218       | BL Lac         | HSP        | ...                  | 1                       |
| 1FHL J1848.5+3219 | 282.125 | 32.322  | B2 1846+32A           | FSRQ           | LSP        | 0.798                | 3                       |
| 1FHL J1849.3+6705 | 282.348 | 67.091  | S4 1849+67            | FSRQ           | LSP        | 0.657                | 1                       |
| 1FHL J1852.3+4853 | 283.082 | 48.888  | S4 1851+48            | FSRQ           | LSP        | 1.250                | 1                       |
| 1FHL J1903.4+5541 | 285.859 | 55.690  | TXS 1902+556          | BL Lac         | ISP        | ...                  | 1                       |
| 1FHL J1910.9-1906 | 287.731 | -19.104 | PMN J1911-1908        | AGU            | ...        | ...                  | 1                       |
| 1FHL J1917.7-1921 | 289.441 | -19.365 | 1H 1914-194           | BL Lac         | HSP        | 0.137                | 1                       |
| 1FHL J1918.1-4109 | 289.538 | -41.165 | PMN J1918-4111        | BL Lac         | ...        | ...                  | 1                       |
| 1FHL J1922.0-1607 | 290.501 | -16.130 | PMN J1921-1607        | BL Lac         | ...        | ...                  | 1                       |
| 1FHL J1926.9+6153 | 291.737 | 61.892  | 1RXS J192649.5+615445 | BL Lac         | HSP        | ...                  | 1                       |
| 1FHL J1931.0+0938 | 292.770 | 9.634   | RX J1931.1+0937       | BL Lac         | HSP        | ...                  | 2                       |
| 1FHL J1936.8-4721 | 294.214 | -47.356 | PMN J1936-4719        | BL Lac         | ...        | 0.265                | 1                       |
| 1FHL J1942.8+1034 | 295.717 | 10.568  | 1RXS J194246.3+103339 | AGU            | HSP        | ...                  | 1                       |
| 1FHL J1958.4-3015 | 299.601 | -30.255 | 1RXS J195815.6-301119 | BL Lac         | HSP        | 0.119                | 1                       |
| 1FHL J2000.0+6509 | 300.007 | 65.158  | 1ES 1959+650          | BL Lac         | HSP        | 0.047                | 1                       |
| 1FHL J2001.1-1752 | 300.278 | -17.868 | PKS 1958-179          | FSRQ           | LSP        | 0.652                | 1                       |
| 1FHL J2001.1+4353 | 300.299 | 43.890  | MAGIC J2001+435       | BL Lac         | ISP        | ...                  | 2                       |
| 1FHL J2009.4-4849 | 302.360 | -48.830 | PKS 2005-489          | BL Lac         | HSP        | 0.071                | 1                       |
| 1FHL J2012.1+4629 | 303.029 | 46.491  | 7C 2010+4619          | BL Lac         | HSP        | ...                  | 1                       |
| 1FHL J2015.8+3710 | 303.961 | 37.175  | VER J2016+372         | FSRQ           | LSP        | 0.859                | 1                       |
| 1FHL J2016.3-0907 | 304.091 | -9.121  | PMN J2016-0903        | BL Lac         | ISP        | 0.367&LowLimit_0.605 | 1                       |
| 1FHL J2018.3+3851 | 304.583 | 38.851  | TXS 2016+386          | AGU            | ...        | ...                  | 1                       |
| 1FHL J2025.8-0734 | 306.466 | -7.577  | PKS 2023-07           | FSRQ           | LSP        | 1.388                | 1                       |
| 1FHL J2031.4+1941 | 307.853 | 19.695  | RX J2030.8+1935       | AGU            | HSP        | ...                  | 1                       |
| 1FHL J2039.2-1045 | 309.801 | -10.757 | TXS 2036-109          | BL Lac         | LSP        | ...                  | 1                       |
| 1FHL J2040.0-7119 | 310.011 | -71.323 | AT20G J204008-711457  | AGU            | ...        | 0.162                | 1                       |

Table 1—Continued

| 1FHL Name         | R.A.    | Decl.   | Assoc.                | Optical Class. | SED Class. | Redshift             | Variability_BayesBlocks |
|-------------------|---------|---------|-----------------------|----------------|------------|----------------------|-------------------------|
| 1FHL J2042.4+2426 | 310.606 | 24.435  | MG2 J204208+2426      | BL Lac         | HSP        | 0.104                | 1                       |
| 1FHL J2056.3-4712 | 314.092 | -47.208 | PKS 2052-47           | FSRQ           | LSP        | 1.489                | 1                       |
| 1FHL J2109.2-6635 | 317.303 | -66.589 | PKS 2104-668          | AGU            | LSP        | ...                  | 1                       |
| 1FHL J2115.6+2935 | 318.908 | 29.597  | B2 2113+29            | FSRQ           | LSP        | 1.514                | 1                       |
| 1FHL J2116.2+3339 | 319.052 | 33.662  | B2 2114+33            | BL Lac         | ISP        | 0.35&1.596           | 1                       |
| 1FHL J2121.0+1901 | 320.263 | 19.032  | OX 131                | FSRQ           | LSP        | 2.180                | 1                       |
| 1FHL J2127.8+3614 | 321.970 | 36.238  | B2 2125+35            | BL Lac         | ISP        | ...                  | 1                       |
| 1FHL J2131.6-0913 | 322.901 | -9.228  | RBS 1752              | BL Lac         | HSP        | 0.449                | 1                       |
| 1FHL J2139.4-4238 | 324.875 | -42.636 | MH 2136-428           | BL Lac         | ISP        | ...                  | 2                       |
| 1FHL J2146.5-1344 | 326.647 | -13.749 | NVSS J214637-134359   | BL Lac         | HSP        | ...                  | 1                       |
| 1FHL J2147.5-7536 | 326.881 | -75.611 | PKS 2142-75           | FSRQ           | LSP        | 1.138                | 1                       |
| 1FHL J2150.2-1413 | 327.572 | -14.223 | TXS 2147-144          | BL Lac         | HSP        | 0.229                | 1                       |
| 1FHL J2158.8-3013 | 329.721 | -30.219 | PKS 2155-304          | BL Lac         | HSP        | 0.116                | 1                       |
| 1FHL J2202.7+4216 | 330.681 | 42.281  | BL Lacertae           | BL Lac         | ISP        | 0.069                | 2                       |
| 1FHL J2203.4+1724 | 330.856 | 17.411  | PKS 2201+171          | FSRQ           | LSP        | 1.076                | 1                       |
| 1FHL J2212.5+2803 | 333.128 | 28.051  | CRATES J2212+2759     | AGU            | ...        | ...                  | 1                       |
| 1FHL J2221.3-5225 | 335.336 | -52.432 | PMN J2221-5224        | BL Lac         | HSP        | ...                  | 1                       |
| 1FHL J2223.4+0104 | 335.860 | 1.070   | NVSS J222329+010226   | BL Lac         | ...        | ...                  | 1                       |
| 1FHL J2236.2+2827 | 339.070 | 28.460  | B2 2234+28A           | BL Lac         | LSP        | 0.795                | 1                       |
| 1FHL J2236.3-1432 | 339.097 | -14.536 | PKS 2233-148          | BL Lac         | LSP        | ...                  | 1                       |
| 1FHL J2244.0+2020 | 341.004 | 20.343  | RGB J2243+203         | BL Lac         | HSP        | ...                  | 1                       |
| 1FHL J2246.9-5205 | 341.734 | -52.088 | 1RXS J224642.0-520638 | AGU            | HSP        | 0.194                | 1                       |
| 1FHL J2247.7+4412 | 341.935 | 44.203  | NVSS J224753+441317   | BL Lac         | HSP        | ...                  | 1                       |
| 1FHL J2250.1+3823 | 342.539 | 38.399  | B3 2247+381           | BL Lac         | HSP        | 0.119                | 1                       |
| 1FHL J2250.7-2811 | 342.698 | -28.187 | PMN J2250-2806        | AGU            | ...        | 0.525                | 2                       |
| 1FHL J2253.9+1608 | 343.477 | 16.146  | 3C 454.3              | FSRQ           | LSP        | 0.859                | 6                       |
| 1FHL J2304.6+3704 | 346.160 | 37.071  | 1RXS J230437.1+370506 | BL Lac         | HSP        | ...                  | 1                       |
| 1FHL J2308.1+1459 | 347.034 | 14.989  | MG1 J230734+1449      | BL Lac         | ...        | 0.503                | 1                       |
| 1FHL J2311.0+3425 | 347.771 | 34.430  | B2 2308+34            | FSRQ           | LSP        | 1.817                | 1                       |
| 1FHL J2314.0+1446 | 348.514 | 14.769  | RGB J2313+147         | BL Lac         | HSP        | 0.163                | 1                       |
| 1FHL J2322.5+3436 | 350.647 | 34.602  | TXS 2320+343          | BL Lac         | HSP        | 0.098                | 1                       |
| 1FHL J2323.8+4210 | 350.962 | 42.171  | 1ES 2321+419          | BL Lac         | HSP        | 0.059&LowLimit_0.268 | 1                       |
| 1FHL J2324.6-4041 | 351.175 | -40.684 | 1ES 2322-409          | BL Lac         | HSP        | 0.174                | 1                       |
| 1FHL J2325.4+3959 | 351.362 | 39.989  | B3 2322+396           | BL Lac         | LSP        | ...                  | 1                       |
| 1FHL J2325.5-4759 | 351.382 | -47.995 | PKS 2322-482          | BL Lac         | ISP        | 0.221                | 1                       |

Table 1—Continued

| 1FHL Name         | R.A.    | Decl.   | Assoc.                | Optical Class. | SED Class. | Redshift | Variability_BayesBlocks |
|-------------------|---------|---------|-----------------------|----------------|------------|----------|-------------------------|
| 1FHL J2329.1+3754 | 352.280 | 37.909  | NVSS J232914+375414   | BL Lac         | HSP        | 0.264    | 1                       |
| 1FHL J2329.2-4957 | 352.304 | -49.959 | PKS 2326-502          | FSRQ           | LSP        | 0.518    | 1                       |
| 1FHL J2334.7+1433 | 353.688 | 14.566  | BZB J2334+1408        | BL Lac         | ...        | ...      | 1                       |
| 1FHL J2341.3+8016 | 355.349 | 80.279  | 1RXS J234051.4+801513 | BL Lac         | HSP        | 0.274    | 1                       |
| 1FHL J2345.0-1556 | 356.261 | -15.937 | PMN J2345-1555        | FSRQ           | LSP        | 0.621    | 3                       |
| 1FHL J2347.0+5142 | 356.759 | 51.705  | 1ES 2344+514          | BL Lac         | HSP        | 0.044    | 1                       |
| 1FHL J2347.2+0707 | 356.806 | 7.123   | CRATES J234639+070503 | AGU            | ISP        | ...      | 1                       |
| 1FHL J2359.2-3037 | 359.812 | -30.618 | H 2356-309            | BL Lac         | HSP        | 0.165    | 1                       |

Note. — R.A. and Decl. are celestial coordinates in J2000 epoch, Assoc. is the name of the associated (or identified) source counterpart, Optical Class. is the optical classification of the AGN, SED class is the SED classification (whenever available), and Variability\_BayesBlocks is the number of Bayesian Blocks (see § 3.3). Four of the sources have two distinct redshifts reported in the literature and their redshifts are listed here separated by the symbol “&”. Three sources have redshifts in the literature that violate the spectroscopic lower limits reported in Shaw et al. (2013); these are listed as “z1 & LowLimit\_z2”. Three 1FHL sources have two associations; names and characteristics of both associated sources are reported separated by the symbol “&”.
